# Supplementary material for: Quantum circuits for simulating linear interferometers
Source: arXiv:2504.16880 source file (2025-09-04)
Supplement: Supplementary file 1 [file supplimental-material.tex]

\documentclass{article}
\usepackage{graphicx} % Required for inserting images
\usepackage[a4paper, total={6in, 11in}]{geometry}

\title{Quantum Circuits for Simulating Linear Interferometers
\date{August, 2025}

\vspace{0.5cm}

\small{\textbf{Supplemental Information}}
}
\author{Hudson Leone}

\begin{document}

\maketitle

\section*{Device Specifications}

All plots and data used in this paper were generated with a Dell Inspiron laptop (model number 15 3525).

\begin{itemize}
    \item \textbf{Memory:} 8.0 GiB
    \item \textbf{Processor:} Processor AMD Ryzen 5 5626u
\end{itemize}

\section*{Compilation Times for Beamsplitter Circuits}

\begin{figure}[h]
    \centering
    \includegraphics[width=0.75\linewidth]{compilation_times.png}
    \caption{
    A scatter plot of compilation times for turning random beamsplitters into quantum circuits. Each \textit{vertical pair} of data points represents a \textit{single} experiment done with a randomly selected beamsplitter.
    Here, the overall compilation time is divided between two subroutines called \texttt{matrix exponentiation} (in blue) and \texttt{circuit synthesis} (in orange). \texttt{Matrix exponentiation} is the amount of time it takes to generate the truncated unitary from the original description of the beamsplitter. \texttt{Circuit synthesis} is amount of time it takes to generate a circuit from this truncated unitary.
    }
    \label{fig:placeholder}
\end{figure}

\end{document}
